# Supplementary material for: An Empirical Study on Ethereum Private Transactions and the Security Implications
Source: arXiv:2208.02858 source file (2022-08-04)
Supplement: Supplementary file 1 [file Appendix-41.tex]

\section{\Pri \Txs Distribution}
% \subsubsection{The count and percentage of \pri \txs.} 
% \mz{the percentage is not by per month, so I removed "per month".}
\bheading{The count and percentage of \pri \txs.} 
    \begin{figure}[t]
    \centering
    \includegraphics[width=1\columnwidth]{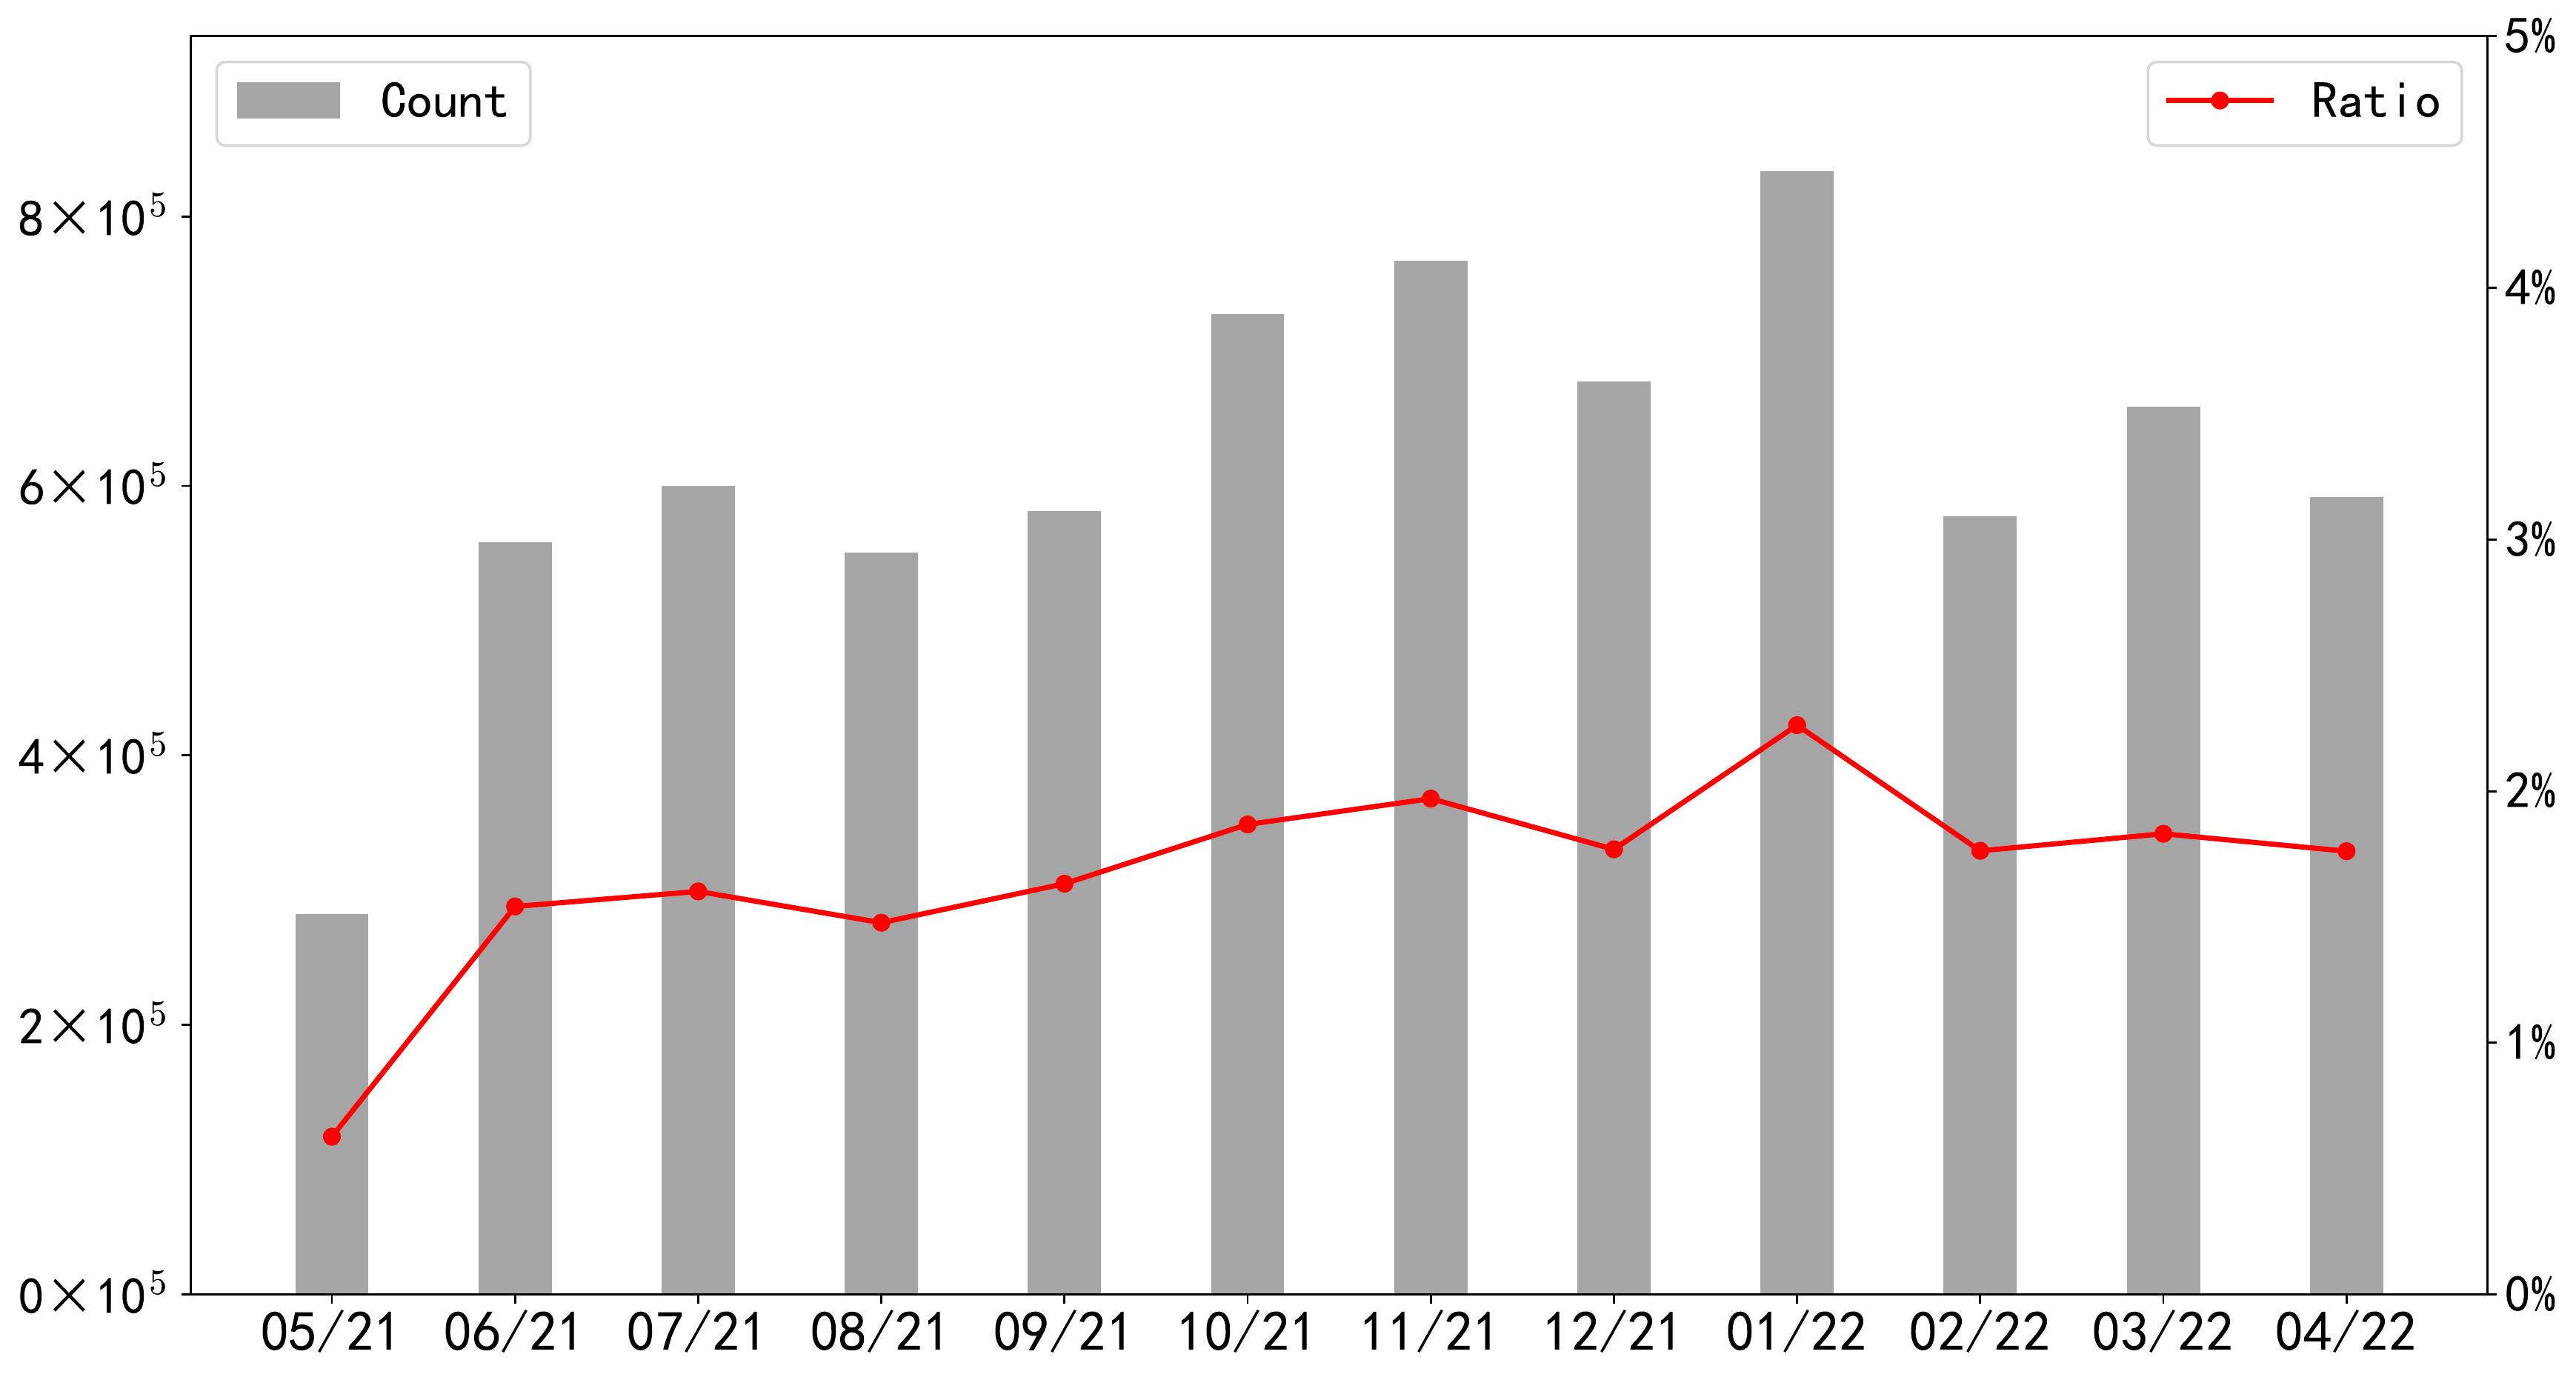}
    \caption{The count and percentage of private transactions per month(x1: \pri \txs per month, x2:percentage in total \txs per month; y: count).} 
    \hfill
    \label{figs:txnum}
    \end{figure}
    % First and foremost, we measure the count of \pri \txs against per month.
    % As shown in ~\figref{figs:txnum}, there are at least 0.28 million \pri \txs every month and around 0.60 million \pri \txs on average per month. 
    % \jn{\figref{figs:txnum} shows the count of \pri \txs against per month.
    % There are at least 0.28 million \pri \txs every month and around 0.60 million \pri \txs on average per month. }
    \figref{figs:txnum} shows the count of \pri \txs against per month.
    There are at least 0.28 million \pri \txs every month and around 0.60 million \pri \txs on average per month. 
    Besides, the percentage of \pri \txs among all the \txs account for 2\% on average per month. 
    Overall, there are not many \pri \txs in the total mined \txs, while the percentage of \pri \txs mostly keeps increasing slightly every month. 
    % \lesson{The count of \pri \txs keeps slightly increasing.}
    % \xz{there are too many observations; can we cut half and only keep the most important/interesting ones?} \mz{ok}

%     \begin{figure}[t]
%     \centering
%     \includegraphics[width=1\columnwidth]{figs/412ptxs/rate_block_px_1.pdf}
%     \caption{The percentage of blocks by the count of \pri \txs within one block (x: the percentage of blocks in this range; y: the range of count of \pri \txs in a block).} 
%     \xl{The data in this figure includes all 2,343,685 blocks from May 1, 2021 to April 30, 2022, of which there are 46\% of the blocks without \pri \txs, and 99.7\% of the blocks with  \pri \txs in the range of [0,20] , and 0.3\% of all blocks with  \pri \txs in the number of 21 $\sim$ 615}
%     \label{figs:rate_alltxperblock}
%     \end{figure}
    
%   % private blocks  
%     \begin{figure}[t]
%     \centering
%     \includegraphics[width=1\columnwidth]{figs/412ptxs/rate_block_px_2.pdf}
%     \caption{The percentage of blocks by the count of \pri \txs within one block (x: the percentage of blocks in this range; y: the range of count of \pri \txs in a block).} 
%     \xl{The data in this figure includes 1,259,251  blocks with \pri \txs from May 1, 2021 to April 30, 2022, of which there are  99.5\% of the blocks with  \pri \txs in the range of [0,20] and 0.5\% of all blocks with  \pri \txs in the number greater than 20(21 $\sim$ 615)}
%     \label{figs:rate_pritxperblock}
%     \end{figure}
\bheading{The distribution of \pri \txs.}
\label{sec:char:dis}
     % all and private blocks  
    \begin{figure}[t]
    \centering
    \includegraphics[width=1\columnwidth]{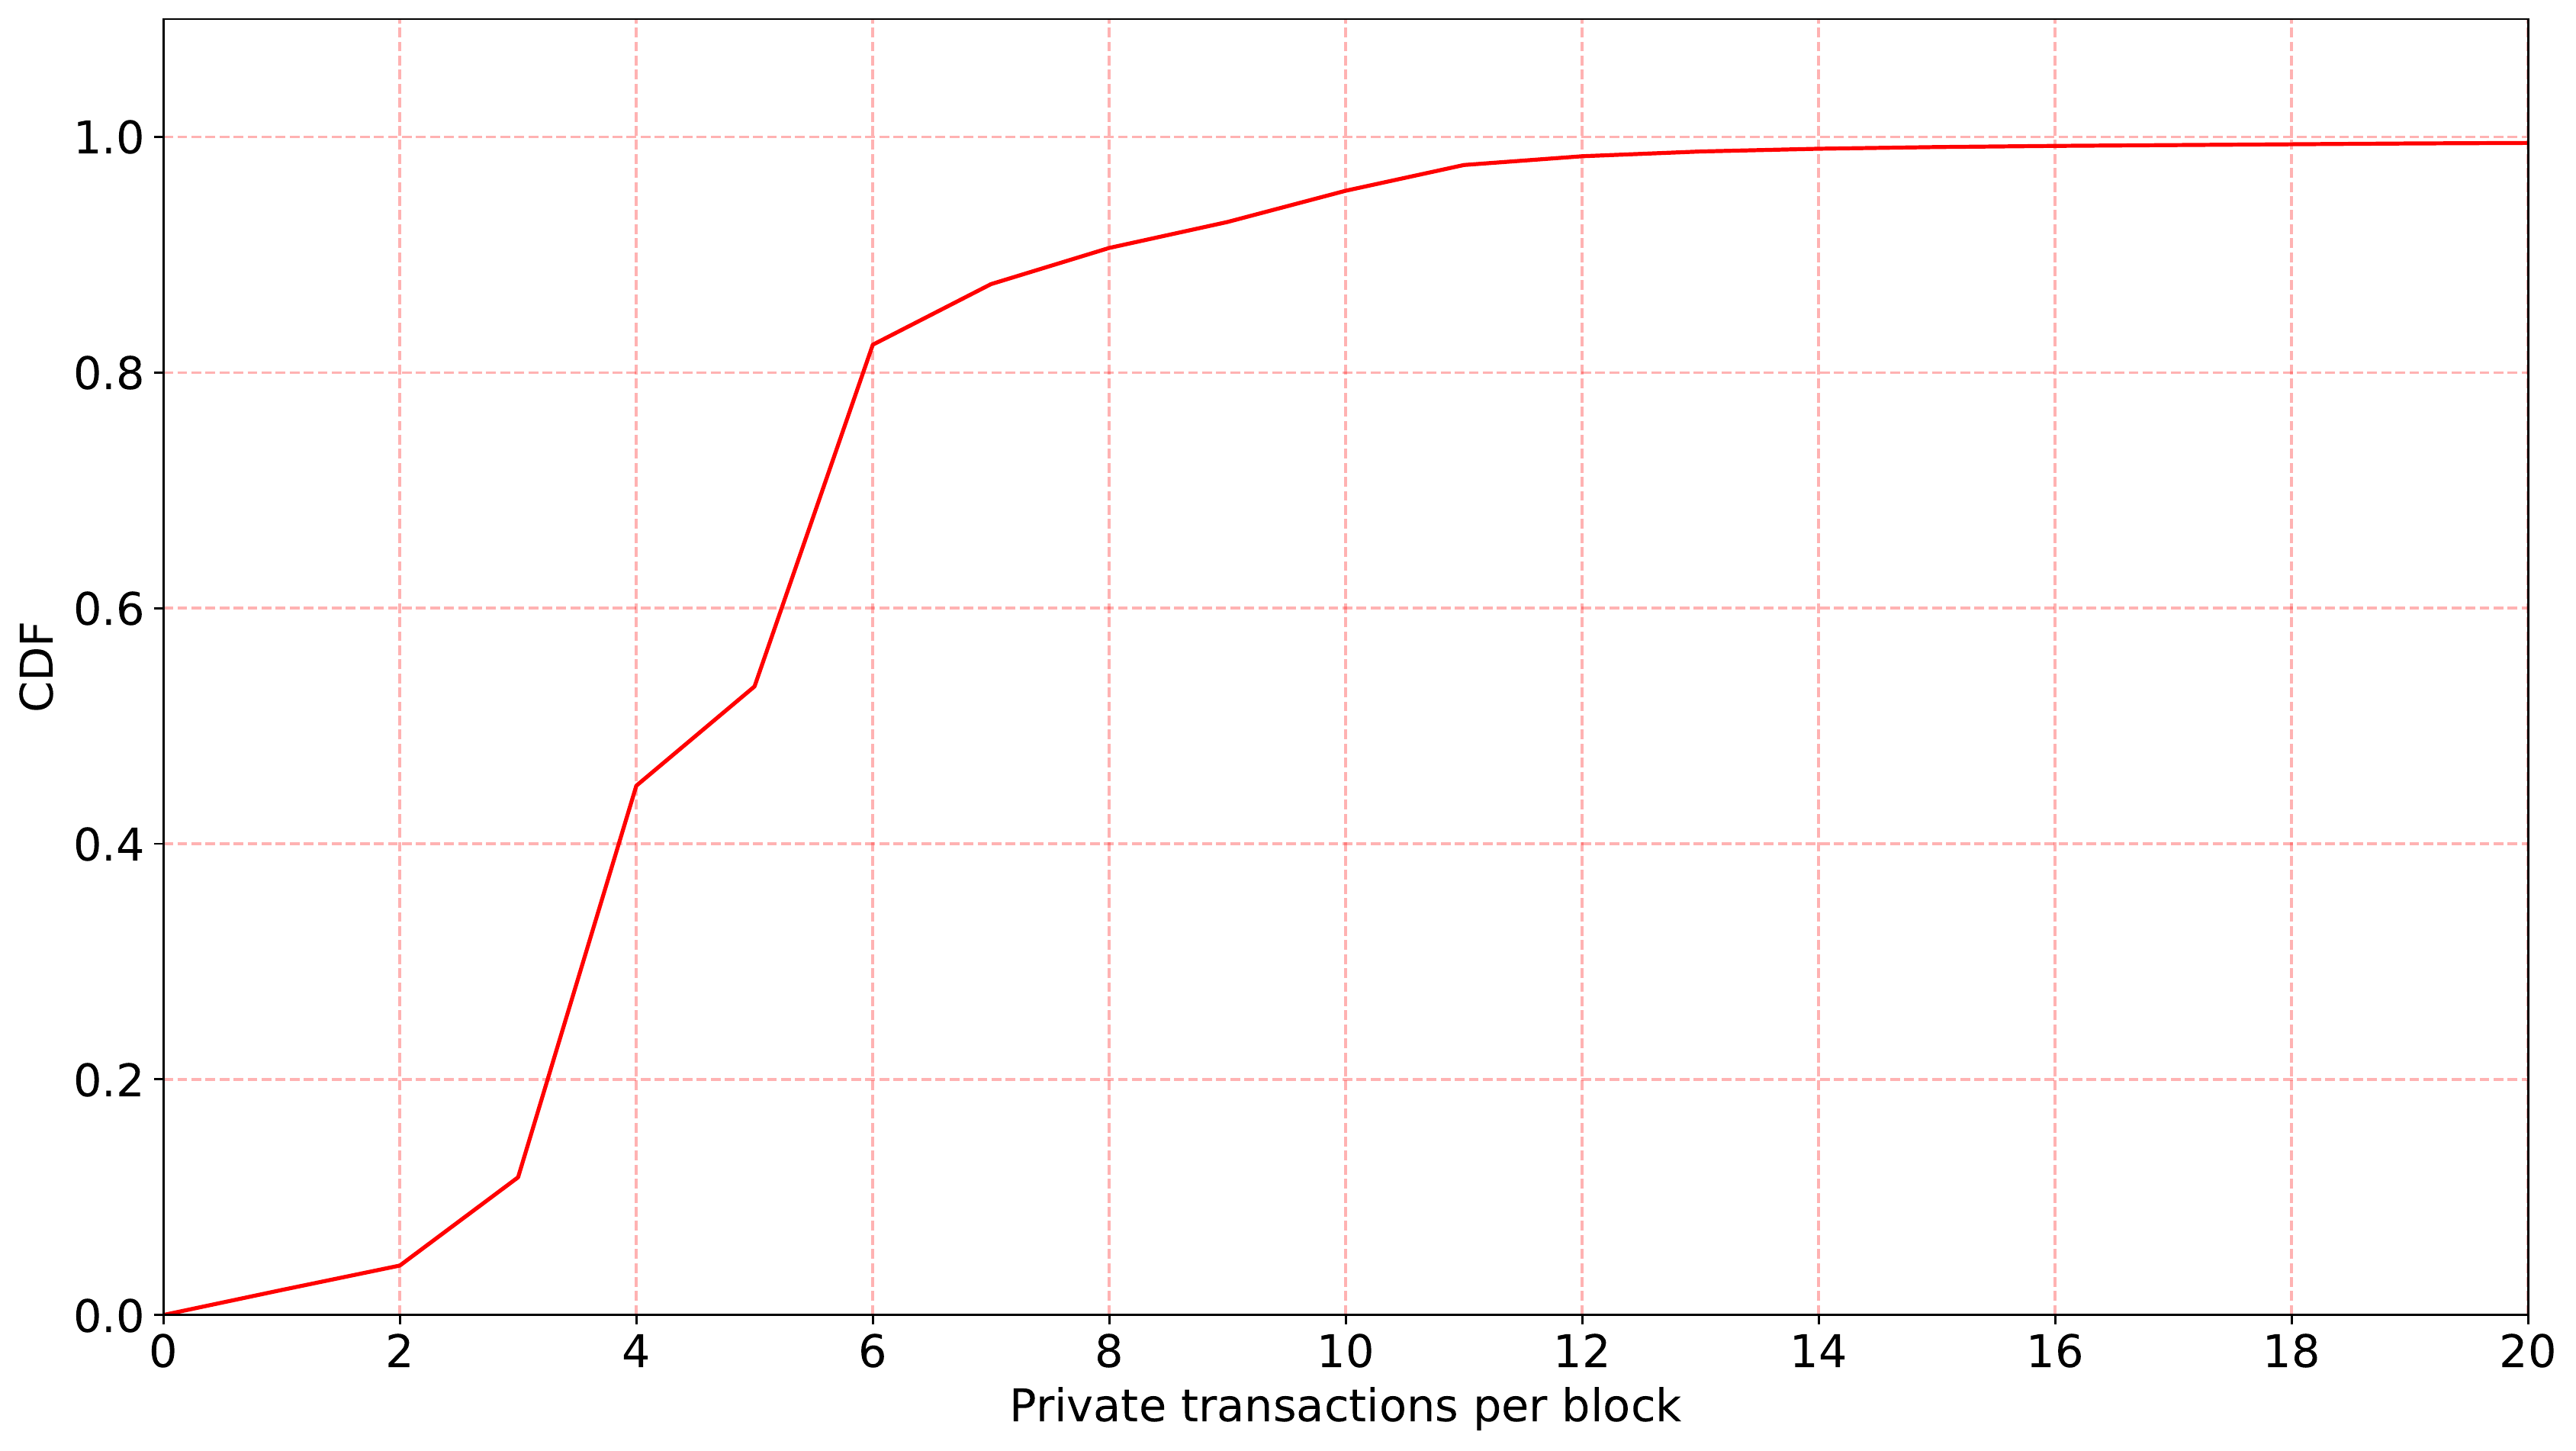}
    \caption{The count of \pri \txs distribution in  blocks with no more than 20 \pri \txs (x: the cumulative percentage of blocks in blocks containing \pri \txs; y: the count of \pri \txs in a single block).} 
    % \xz{what is the point of including two lines? I feel that only keeping one would be good. Also, explain the parts that have count larger then 20; include the numbers in caption}
    \label{figs:rate_mix_perblock}
    \end{figure}
      % all blocks
    \begin{figure}[t]
    \centering
    \includegraphics[width=1\columnwidth]{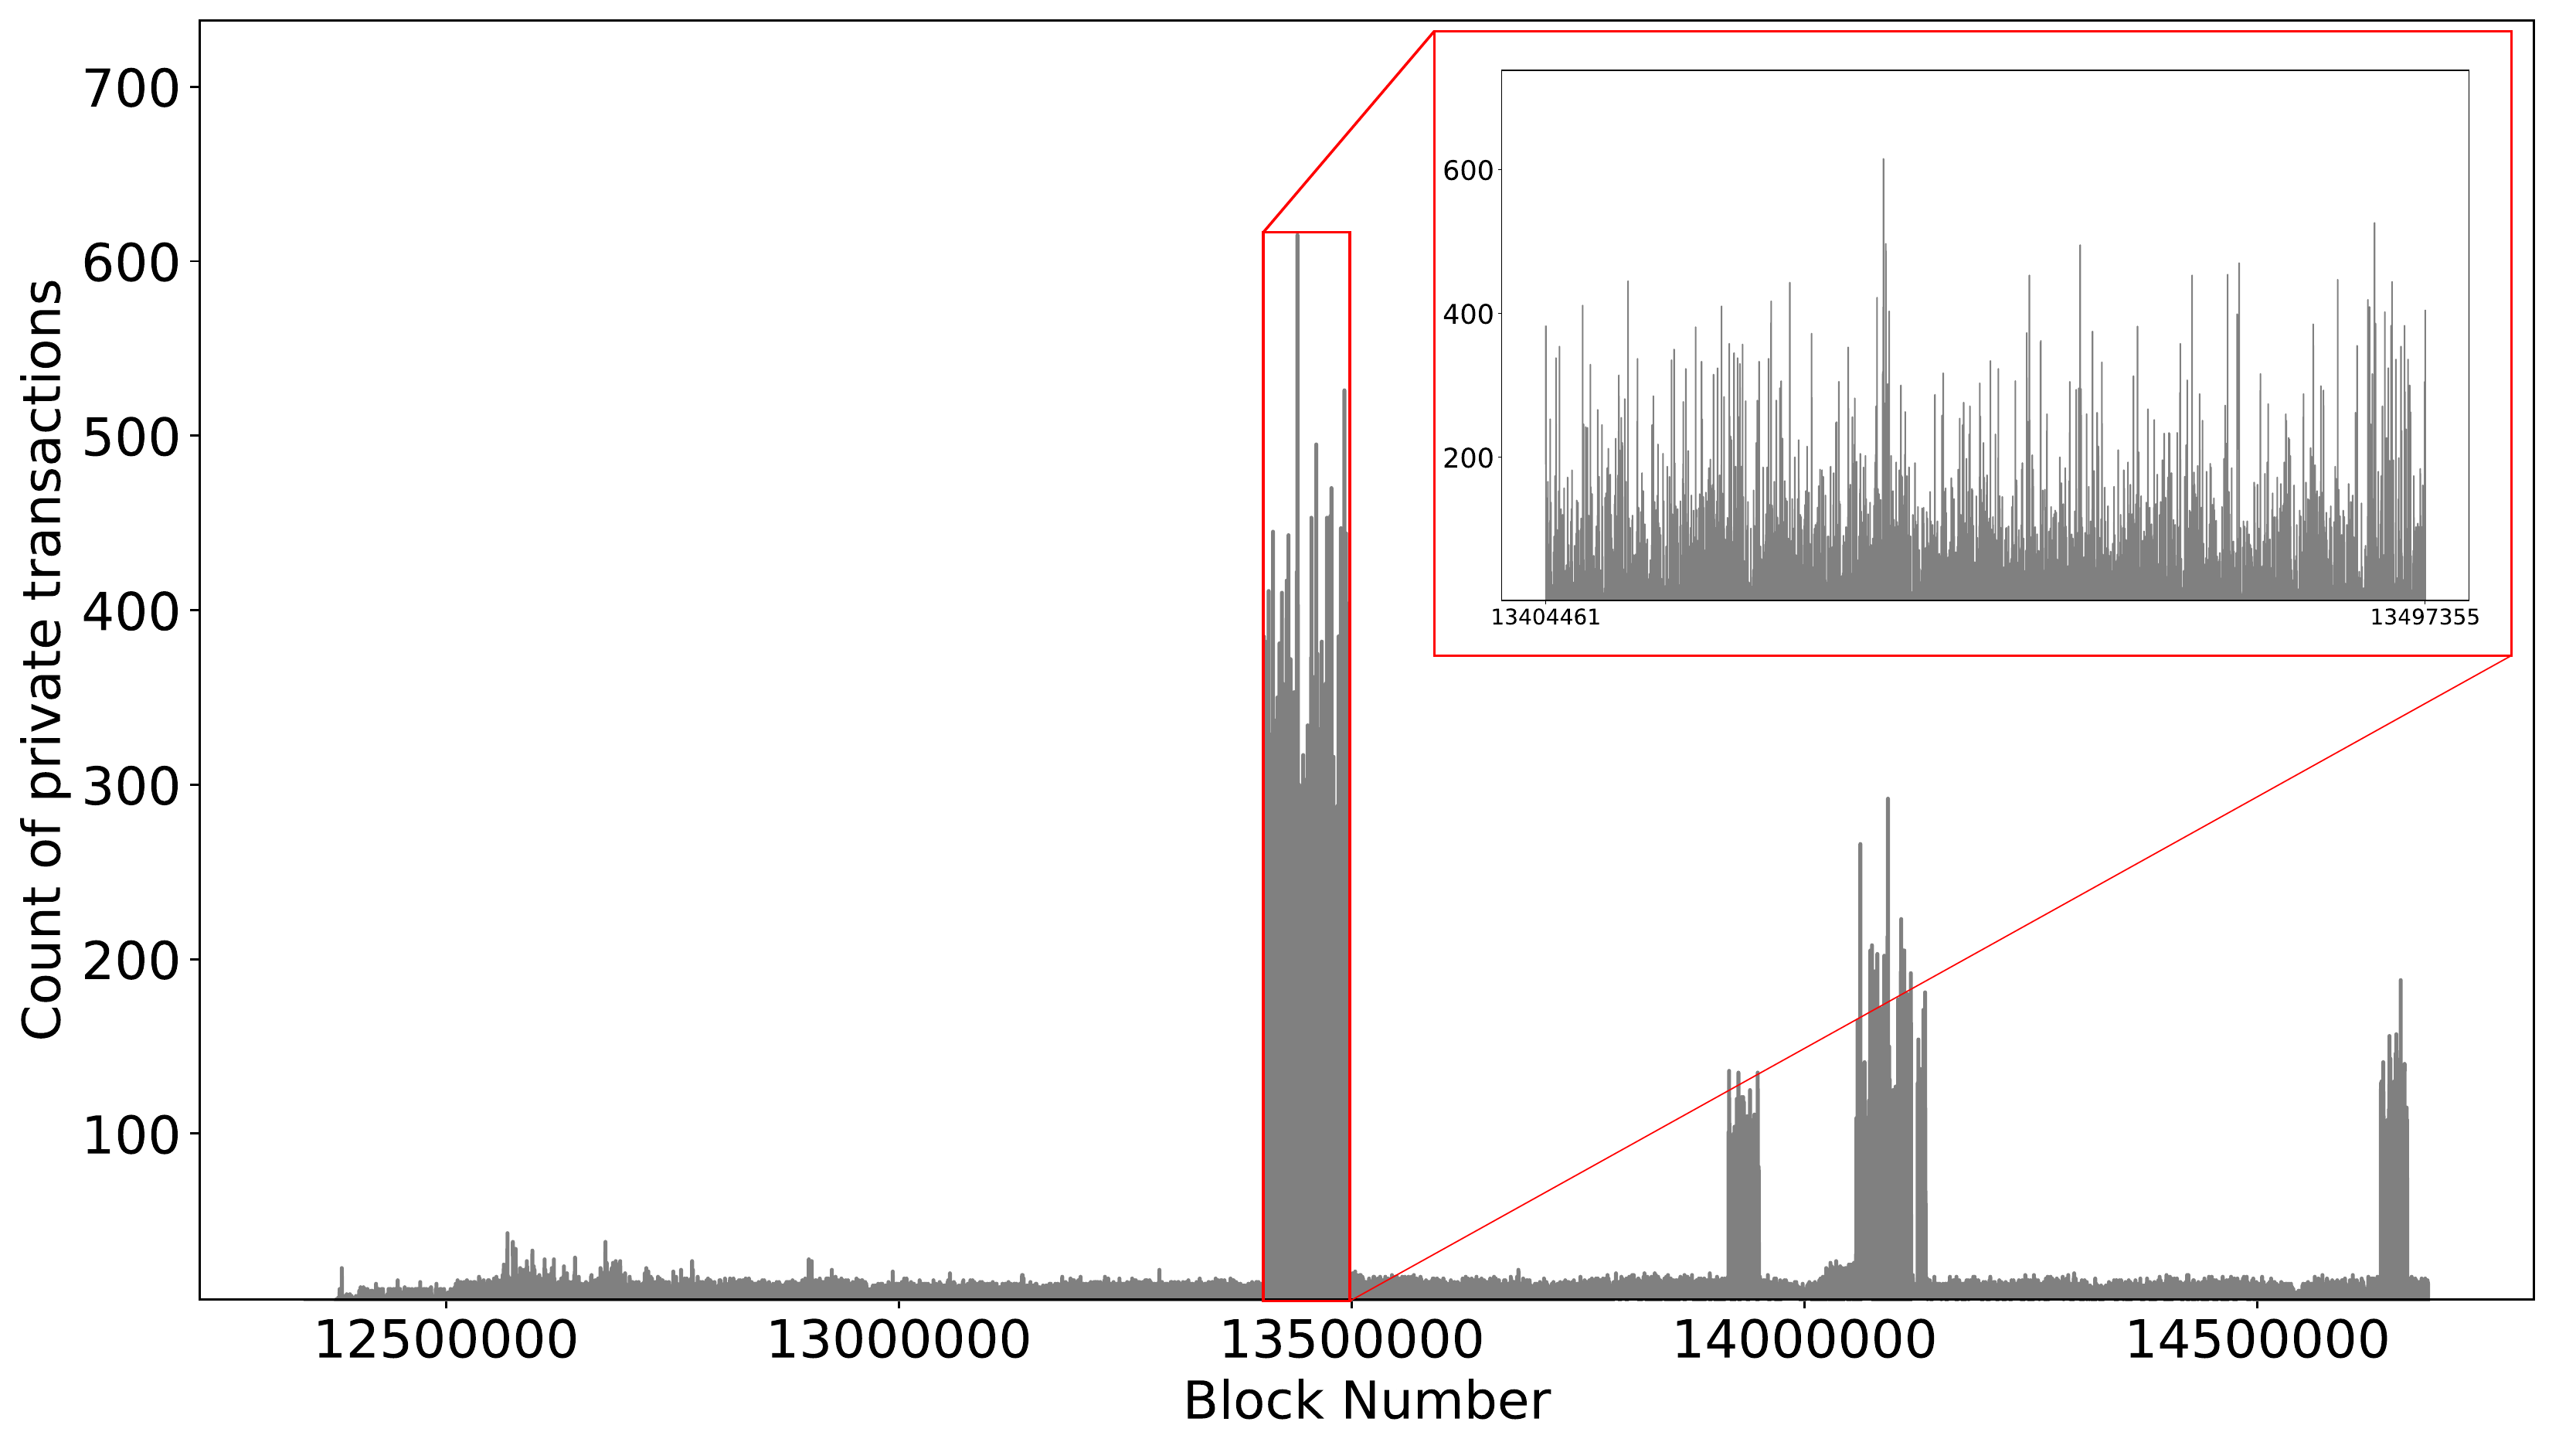}
    \caption{The count of \pri \txs per block (x: the block number; y: the count of \pri \txs in a block).} 
    \label{figs:pritxperblock}
    \end{figure}
     \figref{figs:rate_mix_perblock} plots the count of \pri \txs within a single block distribution that is no more than 20, in terms of  blocks with at least one \pri \tx,
     Specifically, there are 2,343,685 blocks in total, of which 46\% of the blocks contain no \pri \txs. As for the remaining 1,259,251 blocks, there is at least one \pri \tx in every block. Moreover, 99.5\% of these blocks have no more than 20 \pri \txs and 0.5\% have the count of \pri \txs greater than 20 and less than 615.
    % We present the count of \pri \txs against per block in ~\figref{figs:pritxperblock}. 
    % In particular, the block number starts from 12,344,945 and ends with 14,688,626. 
    % Specifically, there is a block 13,440,128 who has more \pri \txs than others. 
    % After a closer examination, the block 13,440,128 contains 615 private transactions, of which more than 580 are miner transfers to the EOA address.
    % In addition, most of the blocks have only a few \pri \txs. 
    % We observe that 93.2\% of blocks have less than 10 \txs and 0.09\% have more than 100 \pri \txs.

%   \lesson{Most (93.2\%) of the blocks have \pri \txs containing less than 10 \pri \txs.}
 
    \bheading{Abnormal count of \pri \txs in some blocks.}
    \figref{figs:pritxperblock} presents the count of \pri \txs against per block and also the blocks in the peek periods. There are four ranges of blocks that seem to have far more \pri \txs than other blocks. The block ranges are [13,404,461 - 13,497,355], [13,926,965 - 13,949,430], [14,057,403 - 14,133,216], and [14,636,264 - 14,664,418], respectively. 
    % ~\figref{figs:pritxperblock} also presents the details of the count of \pri \txs against per block in the biggest peak [13,404,461 - 13,497,355]. 
    We show the details of the biggest peek in the figure.
    In particular, not all of the blocks have far more \pri \txs than others and some blocks have the count of \pri \txs below the average. 
    In particular, we study the blocks with more \pri \txs than others and find that many \pri \txs are used for miners transferring \textit{ETH} to EOAs. Moreover, the other three peeks have the similar patterns.
    
    \lesson{There are four ranges where blocks mine more \pri \txs than average and these \pri \txs are mostly used for transferring money from miners.}

    % \bheading{The positions of \pri \txs inside blocks.}
    % \Pri \txs are usually bundled together to miners and placed at the top of the block. With the data from all the 1,259,251 blocks, we observe that all the \pri \txs are located in front of normal \txs in blocks. The results are expected since \pri \txs are created to race for the opportunities before other \txs. Thus, they should be put in the top positions of the blocks.  
    
    % \lesson{\Pri \txs are placed in front of other normal \txs in blocks. \xz{this is expected}}
